# Supplementary material for: The $GW$ Approximation: A Quantum Chemistry Perspective
Source: arXiv:2311.05351 ancillary file (2024-03-19)
Supplement: Supplementary file 1 [file si.pdf]

# Supporting Information for “The *GW* Approximation: A Quantum Chemistry Perspective”

Antoine Marie,<sup>a)</sup> Abdallah Ammar,<sup>b)</sup> and Pierre-François Loos<sup>c)</sup>

*Laboratoire de Chimie et Physique Quantiques (UMR 5626), Université de Toulouse, CNRS, UPS, France*

This document provides additional information to the accompanying manuscript. The first section follows the outline of Section II of the main document but with more details in the derivation. The second section shows how to compute the matrix elements needed for a *GW* calculation. For more details, we refer the reader to Ref. 1–3 and the references therein.

We adopt the following notations:

- $\mathbf{r}$  represents spatial variables, while  $\mathbf{x}$  represents space-spin variables.
- The integers  $1, 1', 2, 2', \dots$  are shortcut notations. For example, we have  $1 = (\mathbf{x}_1, t_1)$  where  $t_1$  is a time variable and  $\mathbf{x}_1 = (\sigma_1, \mathbf{r}_1)$  is a composite spin-space variable.
- The symbols  $p, q, r, s$  refer to arbitrary spin-orbitals, while  $i, j$  indicate occupied spin-orbitals, and  $a, b$  denote virtual spin-orbitals.

## I. *GW* in theory

The *GW* method aims to provide a detailed description of the electronic structure and spectral properties of materials by utilizing the one-body Green’s function, which is defined as

$$G(11') = (-i) \langle \Psi_0^N | \hat{T} [\hat{\psi}(1) \hat{\psi}^\dagger(1')] | \Psi_0^N \rangle, \quad (1)$$

where  $\Psi_0^N$  is the exact  $N$ -electron ground state and  $\hat{T}$  is the time-ordering operator

$$\hat{T} [\hat{\psi}(1) \hat{\psi}^\dagger(1')] = \Theta(t_1 - t_{1'}) \hat{\psi}(1) \hat{\psi}^\dagger(1') - \Theta(t_{1'} - t_1) \hat{\psi}^\dagger(1') \hat{\psi}(1). \quad (2)$$

Here,  $\Theta$  is the Heaviside function, while  $\hat{\psi}(1)$  and  $\hat{\psi}^\dagger(1')$  represent second-quantized annihilation and creation field operators in the Heisenberg picture, respectively. These operators are defined as follows

$$\hat{\psi}(1) = \hat{\psi}(\mathbf{x}_1 t_1) = e^{i\hat{H}t_1} \hat{\psi}(\mathbf{x}_1) e^{-i\hat{H}t_1}, \quad \hat{\psi}^\dagger(1) = \hat{\psi}^\dagger(\mathbf{x}_1 t_1) = e^{i\hat{H}t_1} \hat{\psi}^\dagger(\mathbf{x}_1) e^{-i\hat{H}t_1}, \quad (3)$$

where  $\hat{\psi}(\mathbf{x})$  and  $\hat{\psi}^\dagger(\mathbf{x})$  are field operators in the Schrödinger picture. They are responsible for, respectively, annihilating and creating a particle with spin  $\sigma$  and position  $\mathbf{r}$ . Here  $\hat{H}$  is the Hamiltonian

$$\hat{H} = \int d(\mathbf{x}_1 \mathbf{x}_{1'}) \hat{\psi}^\dagger(\mathbf{x}_1) h(\mathbf{x}_1 \mathbf{x}_{1'}) \hat{\psi}(\mathbf{x}_{1'}) + \frac{1}{2} \iint d(\mathbf{x}_1 \mathbf{x}_2 \mathbf{x}_{1'} \mathbf{x}_{2'}) \hat{\psi}^\dagger(\mathbf{x}_1) \hat{\psi}^\dagger(\mathbf{x}_2) v(\mathbf{x}_1 \mathbf{x}_2; \mathbf{x}_{1'} \mathbf{x}_{2'}) \hat{\psi}(\mathbf{x}_{2'}) \hat{\psi}(\mathbf{x}_{1'}), \quad (4)$$

where the four-point Coulomb interaction is defined as

$$v(\mathbf{x}_1 \mathbf{x}_2; \mathbf{x}_{1'} \mathbf{x}_{2'}) = \delta(\mathbf{x}_1 - \mathbf{x}_{1'}) \frac{1}{|\mathbf{r}_1 - \mathbf{r}_2|} \delta(\mathbf{x}_2 - \mathbf{x}_{2'}). \quad (5)$$

Because the Hamiltonian is time-independent,  $G(11')$  depends only on the time difference  $t_1 - t_{1'}$ . Inserting the resolution of the identity obtained from the complete spectrum of the  $(N \pm 1)$ -electron systems

$$\sum_S |\Psi_S^{N+1}\rangle \langle \Psi_S^{N+1}| = \hat{I}, \quad \sum_S |\Psi_S^{N-1}\rangle \langle \Psi_S^{N-1}| = \hat{I}, \quad (6)$$

(where  $\hat{I}$  is the identity operator) between the field operators, and then performing the Fourier transform of the one-body Green’s leads to its well-known Lehman representation

$$G(\mathbf{x}_1 \mathbf{x}_{1'}; \omega) = \lim_{\eta \rightarrow 0^+} \sum_S \left[ \frac{\mathcal{I}_S(\mathbf{x}_1) \mathcal{I}_S^*(\mathbf{x}_{1'})}{\omega - (E_0^N - E_S^{N-1}) - i\eta} + \frac{\mathcal{A}_S(\mathbf{x}_1) \mathcal{A}_S^*(\mathbf{x}_{1'})}{\omega - (E_0^{N+1} - E_S^N) + i\eta} \right]. \quad (7)$$

<sup>a)</sup>Electronic mail: [amarie@irsamc.ups-tlse.fr](mailto:amarie@irsamc.ups-tlse.fr)

<sup>b)</sup>Electronic mail: [aammr@irsamc.ups-tlse.fr](mailto:aammr@irsamc.ups-tlse.fr)

<sup>c)</sup>Electronic mail: [loos@irsamc.ups-tlse.fr](mailto:loos@irsamc.ups-tlse.fr)

where  $\eta$  is a positive infinitesimal,  $E_0^N$  is the ground state energy of the  $N$ -electron system,  $E_S^{N+1}$  and  $E_S^{N-1}$  are the excited state energy of the  $(N \pm 1)$ -electron systems, respectively. The numerators are defined as follows

$$\mathcal{I}_S(\mathbf{x}) = \langle \Psi_S^{N-1} | \hat{\psi}(\mathbf{x}) | \Psi_0^N \rangle, \quad \mathcal{A}_S(\mathbf{x}) = \langle \Psi_0^N | \hat{\psi}(\mathbf{x}) | \Psi_S^{N+1} \rangle, \quad (8)$$

and are commonly referred to as the Lehmann amplitudes or Dyson orbitals. The exact expression for  $G$  as given in Eq. (7) can be approximated within the framework of the quasiparticle picture, resulting in the following representation

$$G(\mathbf{x}_1 \mathbf{x}_{1'}; \omega) = \sum_i \frac{\varphi_i(\mathbf{x}_1) \varphi_i^*(\mathbf{x}_{1'})}{\omega - \epsilon_i - i\eta} + \sum_a \frac{\varphi_a(\mathbf{x}_1) \varphi_a^*(\mathbf{x}_{1'})}{\omega - \epsilon_a + i\eta}. \quad (9)$$

In this context,  $\varphi_p$  signifies a complete set of one-electron functions describing quasiparticles, while  $\epsilon_p$  designates the corresponding quasiparticle energies.

### A. Equation of motion for the one-body Green's function

The success of the  $GW$  approximation, as well as other Green's function-based approximations, arises from the ability to compute sufficiently accurate approximations of  $G$  without the need for explicit reference to the wave function  $|\Psi_0^N\rangle$ . This is achieved thanks to a closed set of equations for  $G$ . The derivation of this set commences with an examination of the equation of motion (EOM) for the one-body Green's function. As an initial step toward its formulation, we must derive the EOM for the field operator

$$\begin{aligned} \frac{\partial \hat{\psi}(1)}{\partial t_1} &= \frac{\partial (e^{i\hat{H}t_1} \hat{\psi}(\mathbf{x}_1) e^{-i\hat{H}t_1})}{\partial t_1} = \frac{\partial (e^{i\hat{H}t_1})}{\partial t_1} \hat{\psi}(\mathbf{x}_1) e^{-i\hat{H}t_1} + e^{i\hat{H}t_1} \hat{\psi}(\mathbf{x}_1) \frac{\partial (e^{-i\hat{H}t_1})}{\partial t_1} \\ &= i\hat{H}\hat{\psi}(1) - i\hat{\psi}(1)\hat{H} = -i[\hat{\psi}(1), \hat{H}]. \end{aligned}$$

It can be easily demonstrated that this commutator is expressed as

$$[\hat{\psi}(\mathbf{x}), \hat{H}] = \int d\mathbf{x}_1 v(\mathbf{x}\mathbf{x}_1) \hat{\psi}(\mathbf{x}_1) + \int d\mathbf{x}_2 d\mathbf{x}_1 d\mathbf{x}_2' v(\mathbf{x}\mathbf{x}_2; \mathbf{x}_1 \mathbf{x}_2') \hat{\psi}^\dagger(\mathbf{x}_2) \hat{\psi}(\mathbf{x}_2') \hat{\psi}(\mathbf{x}_1).$$

We are now ready to derive the EOM for the one-body Green's function

$$\begin{aligned} i \frac{\partial G(11')}{\partial t_1} &= \frac{\partial}{\partial t_1} [\Theta(t_1 - t_{1'}) \langle \Psi_0^N | \hat{\psi}(1) \hat{\psi}^\dagger(1') | \Psi_0^N \rangle - \Theta(t_{1'} - t_1) \langle \Psi_0^N | \hat{\psi}^\dagger(1') \hat{\psi}(1) | \Psi_0^N \rangle] \\ &= \delta(t_1 - t_{1'}) \langle \Psi_0^N | \hat{\psi}(1) \hat{\psi}^\dagger(1') | \Psi_0^N \rangle + \delta(t_{1'} - t_1) \langle \Psi_0^N | \hat{\psi}^\dagger(1') \hat{\psi}(1) | \Psi_0^N \rangle \\ &\quad + \Theta(t_1 - t_{1'}) \langle \Psi_0^N | \frac{\partial \hat{\psi}(1)}{\partial t_1} \hat{\psi}^\dagger(1') | \Psi_0^N \rangle - \Theta(t_{1'} - t_1) \langle \Psi_0^N | \hat{\psi}^\dagger(1') \frac{\partial \hat{\psi}(1)}{\partial t_1} | \Psi_0^N \rangle \\ &= \delta(t_1 - t_{1'}) \langle \Psi_0^N | \hat{\psi}(1) \hat{\psi}^\dagger(1') + \hat{\psi}^\dagger(1') \hat{\psi}(1) | \Psi_0^N \rangle \\ &\quad + \Theta(t_1 - t_{1'}) \langle \Psi_0^N | [-i[\hat{\psi}(1), \hat{H}]] \hat{\psi}^\dagger(1') | \Psi_0^N \rangle - \Theta(t_{1'} - t_1) \langle \Psi_0^N | \hat{\psi}^\dagger(1') [-i[\hat{\psi}(1), \hat{H}]] | \Psi_0^N \rangle \\ &= \delta(11') - i \left[ \Theta(t_1 - t_{1'}) \langle \Psi_0^N | \int d\mathbf{x}_3 h(\mathbf{x}_1 \mathbf{x}_3) \hat{\psi}(\mathbf{x}_3 t_1) \hat{\psi}^\dagger(1') | \Psi_0^N \rangle - \Theta(t_{1'} - t_1) \langle \Psi_0^N | \hat{\psi}^\dagger(1') \int d\mathbf{x}_3 h(\mathbf{x}_1 \mathbf{x}_3) \hat{\psi}(\mathbf{x}_3 t_1) | \Psi_0^N \rangle \right] \\ &\quad - i\Theta(t_1 - t_{1'}) \langle \Psi_0^N | \left[ \int d\mathbf{x}_2 d\mathbf{x}_3 d\mathbf{x}_2' v(\mathbf{x}_1 \mathbf{x}_2; \mathbf{x}_3 \mathbf{x}_2') \hat{\psi}^\dagger(\mathbf{x}_2 t_1) \hat{\psi}(\mathbf{x}_2' t_1) \hat{\psi}(\mathbf{x}_3 t_1) \right] \hat{\psi}^\dagger(1') | \Psi_0^N \rangle \\ &\quad + i\Theta(t_{1'} - t_1) \langle \Psi_0^N | \hat{\psi}^\dagger(1') \left[ \int d\mathbf{x}_2 d\mathbf{x}_3 d\mathbf{x}_2' v(\mathbf{x}_1 \mathbf{x}_2; \mathbf{x}_3 \mathbf{x}_2') \hat{\psi}^\dagger(\mathbf{x}_2 t_1) \hat{\psi}(\mathbf{x}_2' t_1) \hat{\psi}(\mathbf{x}_3 t_1) \right] | \Psi_0^N \rangle \\ &= \delta(11') + \int d\mathbf{x}_3 h(\mathbf{x}_1 \mathbf{x}_3) G(\mathbf{x}_3 t_1, 1') - i \int d\mathbf{x}_2 d\mathbf{x}_3 d\mathbf{x}_2' v(\mathbf{x}_1 \mathbf{x}_2; \mathbf{x}_3 \mathbf{x}_2') \\ &\quad \left[ \Theta(t_1 - t_{1'}) \langle \Psi_0^N | \hat{\psi}^\dagger(\mathbf{x}_2 t_1) \hat{\psi}(\mathbf{x}_2' t_1) \hat{\psi}(\mathbf{x}_3 t_1) \hat{\psi}^\dagger(1') | \Psi_0^N \rangle - \Theta(t_{1'} - t_1) \langle \Psi_0^N | \hat{\psi}^\dagger(1') \hat{\psi}^\dagger(\mathbf{x}_2 t_1) \hat{\psi}(\mathbf{x}_2' t_1) \hat{\psi}(\mathbf{x}_3 t_1) | \Psi_0^N \rangle \right] \\ &= \delta(11') + \int d\mathbf{x}_3 h(13) G(31') - i \int d\mathbf{x}_2 d\mathbf{x}_3 d\mathbf{x}_2' v(\mathbf{x}_1 \mathbf{x}_2; \mathbf{x}_3 \mathbf{x}_2') \\ &\quad \left[ \Theta(t_1 - t_{1'}) \langle \Psi_0^N | \hat{\psi}^\dagger(\mathbf{x}_2 t_1) \hat{\psi}(\mathbf{x}_2' t_1) \hat{\psi}(\mathbf{x}_3 t_1) \hat{\psi}^\dagger(1') | \Psi_0^N \rangle - \Theta(t_{1'} - t_1) \langle \Psi_0^N | \hat{\psi}^\dagger(1') \hat{\psi}^\dagger(\mathbf{x}_2 t_1) \hat{\psi}(\mathbf{x}_2' t_1) \hat{\psi}(\mathbf{x}_3 t_1) | \Psi_0^N \rangle \right], \end{aligned}$$

where  $h(12) = \delta(t_1 - t_2) h(\mathbf{x}_1 \mathbf{x}_2)$  and the element  $di \equiv d\mathbf{x}_i dt_i$  represents integration over both time and space. At this point, it is natural to try to use the two latter terms to form the two-body Green's function  $G_2$  which is defined as

$$G_2(12; 1'2') = (-i)^2 \langle \Psi_0^N | \hat{T} [\hat{\psi}(1) \hat{\psi}(2) \hat{\psi}^\dagger(2') \hat{\psi}^\dagger(1')] | \Psi_0^N \rangle. \quad (10)$$

To achieve this, a time-ordering operator is required. However, since three field operators share the same time, the time-ordering operator cannot be unambiguously defined. To overcome this issue, a workaround involves introducing a small time shift using a positive infinitesimal  $\eta$  ( $t_{i+} = t_i + \eta$ ,  $t_{i++} = t_i + 2\eta$ , and so on), as follows

$$\begin{aligned}
& -i \int d(\mathbf{x}_2 \mathbf{x}_3 \mathbf{x}_{2'}) v(\mathbf{x}_1 \mathbf{x}_2; \mathbf{x}_3 \mathbf{x}_{2'}) \\
& \times \lim_{\eta \rightarrow 0^+} \left[ \Theta(t_1 - t_{1'}) \langle \Psi_0^N | \hat{\psi}^\dagger(\mathbf{x}_2 t_{1++}) \hat{\psi}(\mathbf{x}_2' t_{1+}) \hat{\psi}(\mathbf{x}_3 t_1) \hat{\psi}^\dagger(1') | \Psi_0^N \rangle - \Theta(t_{1'} - t_1) \langle \Psi_0^N | \hat{\psi}^\dagger(1') \hat{\psi}^\dagger(\mathbf{x}_2 t_{1++}) \hat{\psi}(\mathbf{x}_2' t_{1+}) \hat{\psi}(\mathbf{x}_3 t_1) | \Psi_0^N \rangle \right] \\
& = -i \int d(\mathbf{x}_2 \mathbf{x}_3 \mathbf{x}_{2'}) v(\mathbf{x}_1 \mathbf{x}_2; \mathbf{x}_3 \mathbf{x}_{2'}) \lim_{\eta \rightarrow 0^+} \langle \Psi_0^N | \hat{T} [\hat{\psi}^\dagger(\mathbf{x}_2 t_{1++}) \hat{\psi}(\mathbf{x}_2' t_{1+}) \hat{\psi}(\mathbf{x}_3 t_1) \hat{\psi}^\dagger(1')] | \Psi_0^N \rangle \\
& = +i \int d(\mathbf{x}_2 \mathbf{x}_3 \mathbf{x}_{2'}) v(\mathbf{x}_1 \mathbf{x}_2; \mathbf{x}_3 \mathbf{x}_{2'}) \lim_{\eta \rightarrow 0^+} \langle \Psi_0^N | \hat{T} [\hat{\psi}(\mathbf{x}_3 t_1) \hat{\psi}(\mathbf{x}_2' t_{1+}) \hat{\psi}^\dagger(\mathbf{x}_2 t_{1++}) \hat{\psi}^\dagger(1')] | \Psi_0^N \rangle \\
& = -i \int d(\mathbf{x}_2 \mathbf{x}_3 \mathbf{x}_{2'}) v(\mathbf{x}_1 \mathbf{x}_2; \mathbf{x}_3 \mathbf{x}_{2'}) \lim_{\eta \rightarrow 0^+} G_2(\mathbf{x}_3 t_1 \mathbf{x}_2' t_{1+}; \mathbf{x}_1' t_1' \mathbf{x}_2 t_{1++}) \\
& = -i \lim_{\eta \rightarrow 0^+} \int d(\mathbf{x}_2 \mathbf{x}_3 \mathbf{x}_{2'}) \int d(t_2 t_3 t_{2'}) v(\mathbf{x}_1 \mathbf{x}_2; \mathbf{x}_3 \mathbf{x}_{2'}) \delta(t_2 - t_1) \delta(t_{2'} - t_1) \delta(t_3 - t_1) G_2(\mathbf{x}_3 t_3 \mathbf{x}_2' t_{2++}; \mathbf{x}_1' t_1' \mathbf{x}_2 t_{2++}) \\
& = -i \lim_{\eta \rightarrow 0^+} \int d(232') v(12; 32') G_2(32'^+; 1'2^{++}).
\end{aligned}$$

The instantaneous Coulomb interaction is defined as follows

$$\begin{aligned}
v(12; 1'2') &= v(\mathbf{x}_1 \mathbf{x}_2; \mathbf{x}_1' \mathbf{x}_2') \delta(t_1 - t_2) \delta(t_1 - t_{1'}) \delta(t_2 - t_{2'}) \\
&= \delta(11') \frac{\delta(t_1 - t_2)}{|\mathbf{r}_1 - \mathbf{r}_2|} \delta(22').
\end{aligned} \tag{11}$$

The EOM of  $G$  becomes

$$\int d3 \left[ i\delta(13) \frac{\partial}{\partial t_3} - h(13) \right] G(31') + \lim_{\eta \rightarrow 0^+} i \int d(232') v(12; 32') G_2(32'^+; 1'2^{++}) = \delta(11'). \tag{12}$$

From now on, we omit the symbol  $\lim_{\eta \rightarrow 0^+}$ .

## B. The self-energy

The non-interacting one-body Green's function is defined as

$$\int d3 \left[ i\delta(13) \frac{\partial}{\partial t_3} - h(13) \right] G_0(31') = \delta(11') \Leftrightarrow \left[ i\delta(13) \frac{\partial}{\partial t_3} - h(13) \right] = G_0^{-1}(13) \tag{13}$$

and its inverse can be identified in the EOM (12). Therefore, if we multiply by  $G_0(71)$  and integrate over 1, we obtain

$$\begin{aligned}
& \int d3 G_0^{-1}(13) G(31') + i \int d(232') v(12; 32') G_2(32'^+; 1'2^{++}) = \delta(11') \\
& \Rightarrow \int d(13) G_0(71) G_0^{-1}(13) G(31') + i \int d(1232') G_0(71) v(12; 32') G_2(32'^+; 1'2^{++}) = \int d1 G_0(71) \delta(11') \\
& \Rightarrow G(11') = G_0(11') - i \int d(232'5) G_0(15) v(52; 32') G_2(32'^+; 1'2^{++}) \\
& \Rightarrow G(11') = G_0(11') + \int d(57) G_0(15) \left[ -i \int d(232'6) v(52; 32') G_2(32'^+; 62^{++}) G^{-1}(67) \right] G(71').
\end{aligned}$$

This equation can be written as the famous Dyson equation,

$$G(11') = G_0(11') + \int d(23) G_0(12) \Sigma(23) G(31'). \tag{14}$$

The total self-energy, encompassing the Hartree-exchange-correlation components, is defined as

$$\Sigma(11') = -i \int d(232'3') v(12; 3'2') G_2(3'2'^+; 32^{++}) G^{-1}(31'). \tag{15}$$

By multiplying Eq. (14) to the right by  $G^{-1}$  and to the left by  $G_0^{-1}$ , integrating and relabeling, it is possible to recast it in the equivalent inverse form

$$G^{-1}(11') = G_0^{-1}(11') - \Sigma(11'). \tag{16}$$

### C. Closed-set equations in terms of the Coulomb potential

The next step is to express the self-energy in terms of  $G$  and the crucial element to do so is the Schwinger relation

$$\left. \frac{\delta G(11'; [U])}{\delta U(2'2)} \right|_{U=0} = -G_2(12; 1'2') + G(11') G(22'). \quad (17)$$

where  $G(11'; [U])$  is the one-body Green's function in presence of an external potential. It is obtained using Eq. (1) as well but with this additional term in the Hamiltonian

$$\hat{U} = \int d\mathbf{x}_2 d\mathbf{x}_2' \hat{\psi}^\dagger(2') U(2'2) \hat{\psi}(2) \quad \text{with} \quad U(2'2) = \Theta(t_2' - t_2) U(\mathbf{r}_2', \mathbf{r}_2; t_2' - t_2). \quad (18)$$

The Schwinger relation allows to express  $G_2$  in terms of the one-body Green's function and its derivative with respect to an external potential  $U$ . For the sake of conciseness, we will omit the explicit dependence on the potential  $U$  in  $G$  and we emphasize that all quantities are evaluated at  $U = 0$ .

The self-energy can now be expressed in terms of  $G$  and its derivative as

$$\begin{aligned} \Sigma(11') &= -i \int d(22'34) v(12; 3'2') \left[ G(3'3) G(2'^+ 2^{++}) - \frac{\delta G(3'3)}{\delta U(2^{++} 2'^+)} \right] G^{-1}(31') \\ &= -i \int d(22') v(12; 1'2') G(2'2^+) + i \int d(22'33') v(12; 3'2') \frac{\delta G(3'3)}{\delta U(2^{++} 2'^+)} G^{-1}(31'). \end{aligned}$$

The first term reduces to the usual Hartree self-energy

$$\begin{aligned} \Sigma_H(11') &= v_H(11') \\ &= -i \int d(22') v(12; 1'2') G(2'2^+) \\ &= -i \int d(\mathbf{x}_2 \mathbf{x}_2') v(\mathbf{x}_1 \mathbf{x}_2; \mathbf{x}_1' \mathbf{x}_2') G(\mathbf{x}_2' \mathbf{x}_2; -\eta). \end{aligned} \quad (19)$$

Therefore, the remaining term encapsulates all the exchange-correlation effects and the self-energy can be rewritten as  $\Sigma(11') = \Sigma_H(11') + \Sigma_{xc}(11')$ . The latter term of the self-energy can be further developed using the following relationship

$$\frac{\delta G(3'3)}{\delta U(2^{++} 2'^+)} = - \int d(56) G(3'5) \frac{\delta G^{-1}(56)}{\delta U(2^{++} 2'^+)} G(63). \quad (20)$$

derived from the definition of the inverse one-body Green's function. This results in

$$\begin{aligned} \Sigma_{xc}(11') &= -i \int d(22'356) v(12; 3'2') G(3'5) \frac{\delta G^{-1}(56)}{\delta U(2^{++} 2'^+)} \delta(61') \\ &= i \int d(22'33') v(12; 32') G(33') \Gamma(3'2'; 1'2^+), \end{aligned}$$

where we have introduced the vertex function

$$\Gamma(12; 1'2') = - \frac{\delta G^{-1}(11')}{\delta U(2'2)}. \quad (21)$$

The final step to obtain a closed set of equations is to derive the Dyson equation for the vertex function using the Dyson equation for  $G$  in presence of an external potential

$$G^{-1}(11') = G_0^{-1}(11') - U(11') - \Sigma(11'), \quad (22)$$

which gives

$$\begin{aligned} \Gamma(12; 1'2') &= \frac{\delta U(11')}{\delta U(2'2)} + \frac{\delta \Sigma(11')}{\delta U(2'2)} \\ &= \delta(12') \delta(1'2) + \int d(33') \frac{\delta \Sigma(11')}{\delta G(33')} \frac{\delta G(33')}{\delta U(2'2)} \\ &= \delta(12') \delta(1'2) - \int d(33') \frac{\delta \Sigma(11')}{\delta G(33')} \int d(44') G(34) \frac{\delta G^{-1}(44')}{\delta U(2'2)} G(4'3') \\ &= \delta(12') \delta(1'2) + \int d(33'44') \Xi(13'; 1'3) G(34) G(4'3') \Gamma(42; 4'2'), \end{aligned}$$

where we have introduced the kernel function

$$\Xi(12; 1'2') = \frac{\delta \Sigma(11')}{\delta G(2'2)}. \quad (23)$$

In summary, the closed set of equations that determine  $G$  can be expressed as follows

$$G(11') = G_0(11') + G_0(12) \Sigma(22') G(2'1'), \quad (24a)$$

$$\Sigma(11') = \Sigma_H(11') + i \int d(22'33') v(12; 32') G(33') \Gamma(3'2'; 1'2^+), \quad (24b)$$

$$\Gamma(12; 1'2') = \delta(12') \delta(1'2) + \int d(33'44') \Xi(13'; 1'3) G(34) G(4'3') \Gamma(42; 4'2'). \quad (24c)$$

#### D. Closed-set equations in terms of the screened Coulomb potential: Hedin's equations

The set derived in the previous section leads to an expansion of the self-energy order by order with respect to the Coulomb interaction  $v$ . Unfortunately, despite being a natural way to build the self-energy, this expansion converges slowly. An alternative set of self-consistent equations, referred to as Hedin's equations, can be derived in a similar manner and yields a closed set of equations in terms of the screened Coulomb potential  $W$  instead of  $v$ . The expansion of the self-energy in terms of  $W$  converges much faster. Hence, this set of equations has been much more successful than the one above. The main idea behind the derivation of Hedin's equation is to use the chain rule with respect to the total classical potential, defined as the sum of the external and Hartree potentials,  $v_{H,\text{ext}}(11') = \Sigma_H(11') + U(11')$ , instead of the sole external potential. The self-energy can be rewritten as  $\Sigma(11') = \Sigma_H(11') + \Sigma_{xc}(11')$ , with

$$\begin{aligned} \Sigma_{xc}(11') &= -i \int d(22'33') v(12; 32') G(33') \frac{\delta G^{-1}(3'1')}{\delta U(2^+2')} \\ &= -i \int d(22'33'44') v(12; 32') G(33') \frac{\delta G^{-1}(3'1')}{\delta v_{H,\text{ext}}(4'4)} \frac{\delta v_{H,\text{ext}}(4'4)}{\delta U(2^+2')} \\ &= i \int d(22'33'44') v(12; 32') G(33') \tilde{\Gamma}(3'4; 1'4') \epsilon^{-1}(4'2'; 42^+), \end{aligned}$$

where

$$\tilde{\Gamma}(12; 1'2') = \frac{\delta G^{-1}(11')}{\delta v_{H,\text{ext}}(2'2)} \quad (25)$$

is irreducible four-point vertex and

$$\epsilon^{-1}(12; 1'2') = \frac{\delta v_{H,\text{ext}}(11')}{\delta U(2'2)} \quad (26)$$

is the inverse dielectric matrix. Upon introduction of the four-point screened interaction

$$W(12; 1'2') = \int d(33') v(13; 1'3') \epsilon^{-1}(23'; 2'3^+), \quad (27)$$

we may write the exchange-correlation self-energy as

$$\Sigma_{xc}(11') = i \int d(22'33') G(33') W(12'; 32) \tilde{\Gamma}(3'2; 1'2'). \quad (28)$$

This can be easily verified to be equivalent to its well-known three-point counterpart.

On the other hand, the expression for the inverse dielectric matrix can be developed as follows

$$\begin{aligned} \epsilon^{-1}(12'; 1'2) &= \frac{\delta (U(11') + \Sigma_H(11'))}{\delta U(22')} \\ &= \delta(12) \delta(1'2) - i \int d(33') v(13; 1'3') L(3'2'; 3^+2). \end{aligned}$$

Here,  $L$  is the electron-hole correlation function (or the four-point reducible polarizability up to a  $-i$  factor)

$$L(12; 1'2') = \frac{\delta G(11')}{\delta U(2'2)}. \quad (29)$$

Using the previous equations, the expression of the screened potential can be expressed as

$$\begin{aligned}
W(12; 1'2') &= \int d(33') v(13; 1'3') \epsilon^{-1}(23'; 2'3^+) \\
&= \int d(33') v(13; 1'3') \left( \delta(3^+2) \delta(3'2') - i \int d(44') v(24; 2'4') L(4'3'; 4^+3^+) \right) \\
&= v(12^-; 1'2') - i \int d(343'4') v(13; 1'3') L(4'3'; 4^+3^+) v(24; 2'4').
\end{aligned} \tag{30}$$

This expression is typically represented in its Dyson form

$$\begin{aligned}
W(12; 1'2') &= v(12^-; 1'2') - i \int d(343'4') v(13; 1'3') \left( \int d(55') \tilde{L}(4'5'; 4^+5) \epsilon^{-1}(53'; 5'3^+) \right) v(24; 2'4') \\
&= v(12^-; 1'2') - i \int d(454'5') W(15; 1'5') \tilde{L}(4'5'; 4^+5) v(24; 2'4'),
\end{aligned} \tag{31}$$

where we have introduced the irreducible four-point polarizability

$$\tilde{L}(12; 1'2') = \frac{\delta G(11')}{\delta v_{H,ext}(2'2)}. \tag{32}$$

which is linked to its reducible counterpart through

$$\begin{aligned}
L(3'2'; 32) &= \int d(44') \frac{\delta G(3'3)}{\delta v_{H,ext}(44')} \frac{\delta v_{H,ext}(44')}{\delta U(22')} \\
&= \int d(44') \tilde{L}(3'4'; 34) \epsilon^{-1}(42'; 4'2) \\
&= \int d(44') \tilde{L}(3'4'; 34) \left[ \delta(24) \delta(2'4') - i \int d(55') v(45; 4'5') L(5'2'; 5^+2) \right] \\
&= \tilde{L}(3'2'; 32) - i \int d(44'55') \tilde{L}(3'4'; 34) v(45; 4'5') L(5'2'; 5^+2).
\end{aligned}$$

The two-point counterpart of  $\tilde{L}$  is often called  $P$ . This equation can be brought to the equivalent form

$$L^{-1}(12; 1'2') = \tilde{L}^{-1}(12; 1'2') + i v(12^-; 1'2'). \tag{33}$$

in a similar way as the Dyson equation of Eq. (16). This identity will be valuable to evaluate the matrix elements of  $L$ . The definition of the inverse of a 4-point function is recalled for the sake of completeness

$$\int d(33') L(13; 1'3') L^{-1}(3'2; 32') = \delta(12') \delta(1'2). \tag{34}$$

The irreducible polarizability  $\tilde{L}$  can be expressed in terms of  $\tilde{\Gamma}$  as well

$$\begin{aligned}
\tilde{L}(12; 1'2') &= \frac{\delta G(11')}{\delta v_{H,ext}(2'2)} \\
&= \int d(33') G(13) \frac{\delta G^{-1}(33')}{\delta v_{H,ext}(2'2)} G(3'1') \\
&= \int d(33') G(13) G(3'1') \tilde{\Gamma}(32; 3'2').
\end{aligned}$$

Hence, the final ingredient missing to close the equations is an equation for the irreducible four-point vertex. The Dyson equation for  $\tilde{\Gamma}$  is exactly the same as the one derived above for its reducible counterpart except that only the exchange-correlation part of the kernel contributes

$$\tilde{\Gamma}(12; 1'2') = \delta(12') \delta(1'2) + \int d(33'44') \Xi_{xc}(13'; 1'3) G(34) G(4'3') \tilde{\Gamma}(42; 4'2'), \tag{35}$$

where

$$\Xi_{xc}(12'; 1'2) = \frac{\delta \Sigma_{xc}(11')}{\delta G(22')}. \quad (36)$$

Finally, the five equations constituting Hedin's equations in the four-point formalism are

$$G(11') = G_0(11') + G_0(12) \Sigma(22') G(2'1'), \quad (37a)$$

$$\Sigma(11') = \Sigma_H(11') + i \int d(22'33') G(33') W(12'; 32) \tilde{\Gamma}(3'2; 1'2'), \quad (37b)$$

$$\tilde{\Gamma}(12; 1'2') = \delta(12') \delta(1'2) + \int d(33'44') \Xi(13'; 1'3) G(34) G(4'3') \tilde{\Gamma}(42; 4'2'), \quad (37c)$$

$$W(12; 1'2') = v(12^-; 1'2') - i \int d(343'4') W(14; 1'4') \tilde{L}(3'4'; 3^+4) v(23; 2'3'), \quad (37d)$$

$$\tilde{L}(12; 1'2') = \int d(33') G(13) G(3'1') \tilde{\Gamma}(32; 3'2'). \quad (37e)$$

### E. GW approximation

The GW approximation is obtained now by considering only the first term in the vertex, i.e.,  $\tilde{\Gamma}(12; 1'2') \approx \delta(12') \delta(1'2)$ . The set of Hedin's equations becomes

$$G(11') = G_0(11') + G_0(12) \Sigma(22') G(2'1'), \quad (38a)$$

$$\Sigma(11') = \Sigma_H(11') + i \int d(22') G(22') W(12'; 21'), \quad (38b)$$

$$W(12; 1'2') = v(12^-; 1'2') - i \int d(343'4') W(14; 1'4') \tilde{L}(3'4'; 3^+4) v(23; 2'3'), \quad (38c)$$

$$\tilde{L}(12; 1'2') = G(12') G(21'). \quad (38d)$$

Note that the last line is consistent with the random-phase approximation (RPA), i.e.,  $\tilde{L}^{GW} = \tilde{L}^{RPA}$ . Instead of the non-interacting  $G_0$ , it is common practice to begin a calculation with a mean-field (Hartree-Fock) starting point

$$\int d3 \left[ i\delta(13) \frac{\partial}{\partial t_3} - F(13) \right] G_{HF}(31') = \delta(11') \Leftrightarrow \left[ i\delta(13) \frac{\partial}{\partial t_3} - F(13) \right] = G_{HF}^{-1}(13). \quad (39)$$

Here,  $F(13) = h(13) + \Sigma_H(13) + \Sigma_x(13)$  represents the Fock operator where  $v_H$  and  $v_x$  are the Hartree and exchange potentials. The expression of the exchange self-energy is recalled for the sake of completeness

$$\Sigma_x(13) = iG(13)v_c(1^+3) \quad (40)$$

Using the Hartree-Fock Green's function  $G_{HF}$ , the Dyson equation becomes

$$G(11') = G_{HF}(11') - \int d(23) G_{HF}(12) \Sigma_c(23) G(31') \Leftrightarrow G^{-1}(11') = G_{HF}^{-1}(11') - \Sigma_c(11') \quad (41)$$

where the correlation self-energy is defined as  $\Sigma_c(11') = \Sigma(11') - \Sigma_H(11') - \Sigma_x(11')$ . Note that the Lehman representation of  $G_{HF}$  [see Eq. (9)] involves the HF orbitals and their corresponding one-electron energies. The latter are the poles of the (approximate) HF Green's function. Hence, they represent approximate ionization potentials and electron affinities which is consistent with Koopmans' theorem.<sup>4</sup>

### II. GW in practice

The aim of this section is to compute the expressions for the matrix elements that need to be implemented in a GW code. It is divided into three parts: the RPA polarizability, the screened interaction, and the self-energy.

#### A. RPA polarizability

The irreducible polarizability in the usual GW approximation is

$$\tilde{L}(12; 1'2') = G(12') G(21'), \quad (42)$$

and the equation for the reducible polarizability derived above is recalled

$$L^{-1}(12; 1'2') = \tilde{L}^{-1}(12; 1'2') + i v(12^-; 1'2').$$

These two polarizabilities depend on three time differences:  $t_1 - t_{1'}$ ,  $t_2 - t_{2'}$ , and  $(t_1 + t_{1'})/2 - (t_2 + t_{2'})/2$ . In Hedin's equations, these polarizabilities are required when  $t_1 = t_{1'}$  and  $t_2 = t_{2'}$ . Therefore, the required quantities depend only on  $\tau_{12} = t_1 - t_2$ .

The Fourier transform of  $\tilde{L}$  with respect to  $\tau_{12}$  reads

$$\begin{aligned} \tilde{L}(\mathbf{x}_1 \mathbf{x}_2; \mathbf{x}_{1'} \mathbf{x}_{2'}; \omega) &= \int d\tau_{12} e^{i\omega\tau_{12}} \tilde{L}(\mathbf{x}_1 \mathbf{x}_2; \mathbf{x}_{1'} \mathbf{x}_{2'}; \tau_{12}) \\ &= \int d\tau_{12} e^{i\omega\tau} G(\mathbf{x}_1 \mathbf{x}_{2'}; \tau_{12}) G(\mathbf{x}_2 \mathbf{x}_{1'}; -\tau_{12}) \\ &= \int d\tau_{12} e^{i\omega\tau_{12}} \int \frac{d\omega'}{2\pi} e^{-i\omega'(+\tau_{12})} G(\mathbf{x}_1 \mathbf{x}_{2'}; \omega') \int \frac{d\omega''}{2\pi} e^{-i\omega''(-\tau_{12})} G(\mathbf{x}_2 \mathbf{x}_{1'}; \omega'') \\ &= \int \frac{d\omega'}{2\pi} G(\mathbf{x}_1 \mathbf{x}_{2'}; \omega') \int \frac{d\omega''}{2\pi} G(\mathbf{x}_2 \mathbf{x}_{1'}; \omega'') \underbrace{\int d\tau_{12} e^{i(\omega - \omega' + \omega'')\tau_{12}}}_{2\pi \delta(\omega - \omega' + \omega'')} \\ &= \int \frac{d\omega'}{2\pi} G(\mathbf{x}_1 \mathbf{x}_{2'}; \omega') G(\mathbf{x}_2 \mathbf{x}_{1'}; \omega' - \omega). \end{aligned}$$

By using the Lehmann representation of the one-body Green's function [see Eq. (9)], we get

$$\begin{aligned} 2\pi \tilde{L}(x_1, x_2; x_{1'}, x_{2'}; \omega) &= \int d\omega' \left( \sum_i \frac{\varphi_i(\mathbf{x}_1) \varphi_i^*(\mathbf{x}_{2'})}{\omega' - (\epsilon_i + i\eta)} + \sum_a \frac{\varphi_a(\mathbf{x}_1) \varphi_a^*(\mathbf{x}_{2'})}{\omega' - (\epsilon_a - i\eta)} \right) \left( \sum_j \frac{\varphi_j(\mathbf{x}_2) \varphi_j^*(\mathbf{x}_{1'})}{\omega' - \omega - (\epsilon_j + i\eta)} + \sum_b \frac{\varphi_b(\mathbf{x}_2) \varphi_b^*(\mathbf{x}_{1'})}{\omega' - \omega - (\epsilon_b - i\eta)} \right) \\ &= \int d\omega' \sum_{ij} \frac{\varphi_i(\mathbf{x}_1) \varphi_i^*(\mathbf{x}_{2'}) \varphi_j(\mathbf{x}_2) \varphi_j^*(\mathbf{x}_{1'})}{(\omega' - (\epsilon_i + i\eta))(\omega' - (\omega + \epsilon_j + i\eta))} + \int d\omega' \sum_{ib} \frac{\varphi_i(\mathbf{x}_1) \varphi_i^*(\mathbf{x}_{2'}) \varphi_b(\mathbf{x}_2) \varphi_b^*(\mathbf{x}_{1'})}{(\omega' - (\epsilon_i + i\eta))(\omega' - (\omega + \epsilon_b - i\eta))} \\ &+ \int d\omega' \sum_{aj} \frac{\varphi_a(\mathbf{x}_1) \varphi_a^*(\mathbf{x}_{2'}) \varphi_j(\mathbf{x}_2) \varphi_j^*(\mathbf{x}_{1'})}{(\omega' - (\epsilon_a - i\eta))(\omega' - (\omega + \epsilon_j + i\eta))} + \int d\omega' \sum_{ab} \frac{\varphi_a(\mathbf{x}_1) \varphi_a^*(\mathbf{x}_{2'}) \varphi_b(\mathbf{x}_2) \varphi_b^*(\mathbf{x}_{1'})}{(\omega' - (\epsilon_a - i\eta))(\omega' - (\omega + \epsilon_b - i\eta))} \\ &= \int_{C^+} d\omega' \sum_{ib} \frac{\varphi_i(\mathbf{x}_1) \varphi_i^*(\mathbf{x}_{2'}) \varphi_b(\mathbf{x}_2) \varphi_b^*(\mathbf{x}_{1'})}{(\omega' - (\epsilon_i + i\eta))(\omega' - (\omega + \epsilon_b - i\eta))} - \int_{C^-} d\omega' \sum_{aj} \frac{\varphi_a(\mathbf{x}_1) \varphi_a^*(\mathbf{x}_{2'}) \varphi_j(\mathbf{x}_2) \varphi_j^*(\mathbf{x}_{1'})}{(\omega' - (\epsilon_a - i\eta))(\omega' - (\omega + \epsilon_j + i\eta))}. \end{aligned}$$

In the preceding expression, the integration over the  $ij$  ( $ab$ ) terms vanishes as all the poles reside in the upper (lower) part of the complex plane.  $C^+$  and  $C^-$  correspond to the contours drawn in Fig. 1, each extending to an infinite radius. The integration over

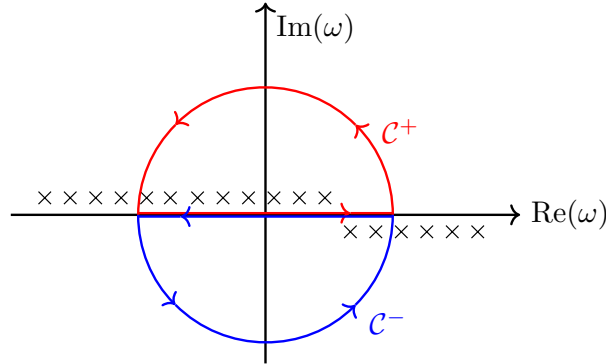

FIG. 1: Integration contours in the complex plane.

these contours leads to

$$\tilde{L}(\mathbf{x}_1 \mathbf{x}_2; \mathbf{x}_{1'} \mathbf{x}_{2'}; \omega) = i \sum_{ia} \left[ \frac{\varphi_a(\mathbf{x}_1) \varphi_a^*(\mathbf{x}_{2'}) \varphi_i(\mathbf{x}_2) \varphi_i^*(\mathbf{x}_{1'})}{\omega - (\epsilon_a - \epsilon_i - 2i\eta)} - \frac{\varphi_i(\mathbf{x}_1) \varphi_i^*(\mathbf{x}_{2'}) \varphi_a(\mathbf{x}_2) \varphi_a^*(\mathbf{x}_{1'})}{\omega - (\epsilon_i - \epsilon_a + 2i\eta)} \right]. \quad (43)$$

The stage is now set to compute the matrix elements of the irreducible polarizability defined as

$$\begin{aligned}\tilde{L}_{pqrs}(\omega) &= \int d\mathbf{x}_1 d\mathbf{x}_2 d\mathbf{x}_{1'} d\mathbf{x}_{2'} \tilde{L}(\mathbf{x}_1 \mathbf{x}_2; \mathbf{x}_{1'} \mathbf{x}_{2'}) \varphi_p^*(\mathbf{x}_1) \varphi_q^*(\mathbf{x}_2) \varphi_r(\mathbf{x}_{1'}) \varphi_s(\mathbf{x}_{2'}) \\ &= i \sum_{ia} \frac{\delta_{pa} \delta_{qi} \delta_{ri} \delta_{sa}}{\omega - (\epsilon_a - \epsilon_i - 2i\eta)} - i \sum_{ia} \frac{\delta_{pi} \delta_{qa} \delta_{ra} \delta_{si}}{\omega - (\epsilon_i - \epsilon_a + 2i\eta)}.\end{aligned}$$

Therefore, the associated matrix  $\tilde{L}(\omega)$  can be written as a diagonal matrix by choosing the right pair of indices

$$\tilde{L}_{rp,qs}(\omega) = i \sum_{ia} \frac{\delta_{psa} \delta_{qri}}{\omega - (\epsilon_a - \epsilon_i - 2i\eta)} - i \sum_{ia} \frac{\delta_{psi} \delta_{qra}}{\omega - (\epsilon_i - \epsilon_a + 2i\eta)}, \quad (44)$$

where  $\delta_{pqr} = \delta_{pq} \delta_{qr}$ . In matrix representation, this expression is equivalent to representing the matrix  $\tilde{L}(\omega)$  in the space of single excitations (and deexcitations) as

$$\tilde{L}(\omega) = \left[ i \begin{pmatrix} \Delta\epsilon & \mathbf{0} \\ \mathbf{0} & \Delta\epsilon \end{pmatrix} - i \omega \begin{pmatrix} \mathbf{1} & \mathbf{0} \\ \mathbf{0} & -\mathbf{1} \end{pmatrix} \right]^{-1},$$

where  $\mathbf{1}$  is the identity matrix and  $\Delta\epsilon_{ia,jb} = (\epsilon_a - \epsilon_i) \delta_{ij} \delta_{ab}$ .

The Fourier transform of the inverse of the reducible polarizability is straightforward

$$L^{-1}(\mathbf{x}_1 \mathbf{x}_2; \mathbf{x}_{1'} \mathbf{x}_{2'}; \omega) = \tilde{L}^{-1}(\mathbf{x}_1 \mathbf{x}_2; \mathbf{x}_{1'} \mathbf{x}_{2'}; \omega) + i v(\mathbf{x}_1 \mathbf{x}_2; \mathbf{x}_{1'} \mathbf{x}_{2'}).$$

Then, the matrix elements of the inverse of the reducible polarizability are obtained as

$$i L_{rp,qs}^{-1}(\omega) = i \tilde{L}_{rp,qs}^{-1}(\omega) - v_{rp,qs}. \quad (45)$$

The matrix elements of the four-point Coulomb operator are

$$\begin{aligned}v_{rp,qs} &= \int d\mathbf{x}_1 d\mathbf{x}_2 d\mathbf{x}_{1'} d\mathbf{x}_{2'} v(\mathbf{x}_1 \mathbf{x}_2; \mathbf{x}_{1'} \mathbf{x}_{2'}) \varphi_p^*(\mathbf{x}_1) \varphi_q^*(\mathbf{x}_2) \varphi_r(\mathbf{x}_{1'}) \varphi_s(\mathbf{x}_{2'}) \\ &= \langle pq|rs \rangle\end{aligned} \quad (46)$$

where

$$\langle pq|rs \rangle = \iint \frac{\varphi_p^*(\mathbf{x}_1) \varphi_q^*(\mathbf{x}_2) \varphi_r(\mathbf{x}_1) \varphi_s(\mathbf{x}_2)}{|\mathbf{r}_1 - \mathbf{r}_2|} d\mathbf{x}_1 d\mathbf{x}_2 \quad (47)$$

are the bare two-electron integrals in the spin-orbital basis. In matrix notation, we obtain

$$i L^{-1}(\omega) = i \tilde{L}^{-1}(\omega) - v = i \left[ i \begin{pmatrix} \Delta\epsilon & \mathbf{0} \\ \mathbf{0} & \Delta\epsilon \end{pmatrix} - i \omega \begin{pmatrix} \mathbf{1} & \mathbf{0} \\ \mathbf{0} & -\mathbf{1} \end{pmatrix} \right] - v = -\mathcal{M} \cdot [\mathcal{H} - \omega \mathbf{1}],$$

where the (unitary) metric matrix  $\mathcal{M}$  and the non-Hermitian matrix  $\mathcal{H}$  are given by

$$\mathcal{M} = \mathcal{M}^{-1} = \begin{pmatrix} \mathbf{1} & \mathbf{0} \\ \mathbf{0} & -\mathbf{1} \end{pmatrix}, \quad \mathcal{H} = \begin{pmatrix} \mathbf{A} & \mathbf{B} \\ -\mathbf{B}^* & -\mathbf{A}^* \end{pmatrix}, \quad (48)$$

such that

$$A_{ia,jb} = (\epsilon_a - \epsilon_i) \delta_{ij} \delta_{ab} + \langle a|j|ib \rangle, \quad B_{ia,jb} = \langle ab|i|j \rangle. \quad (49)$$

The properties of the Coulomb interaction imply that  $\mathbf{B}$  is symmetric and  $\mathbf{A}$  is Hermitian

$$B_{ia,jb} = B_{jb,ia} \Leftrightarrow \mathbf{B}^\top = \mathbf{B}, \quad A_{ia,jb} = A_{jb,ia}^* \Leftrightarrow \mathbf{A}^\dagger = \mathbf{A}. \quad (50)$$

Therefore, one can find the expression of  $L(\omega)$  by using the eigendecomposition of  $\mathcal{H}$ . Let  $\mathcal{L}$  and  $\mathcal{R}$  be the left- and right-eigenvectors of  $\mathcal{H}$

$$\mathcal{H} \cdot \mathcal{R} = \mathcal{R} \cdot \mathcal{E}, \quad \mathcal{H}^\dagger \cdot \mathcal{L} = \mathcal{L} \cdot \mathcal{E}, \quad (51)$$

with the bi-orthonormality condition  $\mathcal{L}^\dagger \cdot \mathcal{R} = \mathbf{1}$ . These eigenvectors allow to decompose the matrix  $\mathcal{H}$  as  $\mathcal{H} = \mathcal{R} \cdot \mathcal{E} \cdot \mathcal{L}^\dagger$ . Thus,

$$\mathbf{i} L^{-1}(\omega) = -\mathcal{M} \cdot [\mathcal{H} - \omega \mathbf{1}] = -\mathcal{M} \cdot [\mathcal{R} \cdot \mathcal{E} \cdot \mathcal{L}^\dagger - \omega \mathcal{R} \cdot \mathcal{L}^\dagger] = -\mathcal{M} \cdot \mathcal{R} \cdot [\mathcal{E} - \omega \mathbf{1}] \cdot \mathcal{L}^\dagger,$$

and we obtain its inverse as

$$\mathbf{i} L(\omega) = \mathcal{R} \cdot [\mathcal{E} - \omega \mathbf{1}]^{-1} \cdot \mathcal{L}^\dagger \cdot \mathcal{M}.$$

The matrix  $\mathcal{H}$  exhibits the well-known structure typically encountered in linear response equations, known as Casida equations. The computation of eigenvectors is reduced to determine two distinct blocks, denoted as  $X$  and  $Y$ :

$$\mathcal{R} = \begin{pmatrix} X & Y^* \\ Y & X^* \end{pmatrix}, \quad \mathcal{L} = \begin{pmatrix} X & -Y^* \\ -Y & X^* \end{pmatrix}, \quad (52)$$

where the normalization constraint is simplified to the two conditions:

$$X^\dagger \cdot X - Y^\dagger \cdot Y = \mathbf{1}, \quad X^\top \cdot Y - Y^\top \cdot X = \mathbf{0}. \quad (53)$$

On the other hand, the eigenvalues of  $\mathcal{H}$  are solely determined by a single diagonal block, denoted as  $\Omega$  and assumed to be real-valued

$$\mathcal{E} = \begin{pmatrix} \Omega & \mathbf{0} \\ \mathbf{0} & -\Omega \end{pmatrix}. \quad (54)$$

Hence, the matrix  $L(\omega)$  is entirely determined by the three blocks  $\Omega$ ,  $X$ , and  $Y$

$$\begin{aligned} \mathbf{i} L(\omega) &= \begin{pmatrix} X & Y^* \\ Y & X^* \end{pmatrix} \cdot \begin{pmatrix} [\Omega - \omega \mathbf{1}]^{-1} & \mathbf{0} \\ \mathbf{0} & -[\Omega + \omega \mathbf{1}]^{-1} \end{pmatrix} \cdot \begin{pmatrix} X^\dagger & -Y^\dagger \\ -Y^\top & X^\top \end{pmatrix} \cdot \begin{pmatrix} \mathbf{1} & \mathbf{0} \\ \mathbf{0} & -\mathbf{1} \end{pmatrix} \\ &= \begin{pmatrix} X \cdot [\Omega - \omega \mathbf{1}]^{-1} \cdot X^\dagger + Y^* \cdot [\Omega + \omega \mathbf{1}]^{-1} \cdot Y^\top & X \cdot [\Omega - \omega \mathbf{1}]^{-1} \cdot Y^\dagger + Y^* \cdot [\Omega + \omega \mathbf{1}]^{-1} \cdot X^\top \\ Y \cdot [\Omega - \omega \mathbf{1}]^{-1} \cdot X^\dagger + X^* \cdot [\Omega + \omega \mathbf{1}]^{-1} \cdot Y^\top & Y \cdot [\Omega - \omega \mathbf{1}]^{-1} \cdot Y^\dagger + X^* \cdot [\Omega + \omega \mathbf{1}]^{-1} \cdot X^\top \end{pmatrix} \\ &= \mathbf{i} \begin{pmatrix} L^I(\omega) & L^{II}(\omega) \\ L^{III}(\omega) & L^{IV}(\omega) \end{pmatrix}, \end{aligned}$$

where the four blocks are defined as

$$\mathbf{i} L_{ia,jb}^I(\omega) = \sum_m \left[ -\frac{X_{ia,m} X_{jb,m}^*}{\omega - \Omega_m + i\eta} + \frac{Y_{ia,m}^* Y_{jb,m}}{\omega + \Omega_m - i\eta} \right], \quad \mathbf{i} L_{ia,jb}^{II}(\omega) = \sum_m \left[ -\frac{X_{ia,m} Y_{jb,m}^*}{\omega - \Omega_m + i\eta} + \frac{Y_{ia,m}^* X_{jb,m}}{\omega + \Omega_m - i\eta} \right], \quad (55)$$

$$\mathbf{i} L_{ia,jb}^{III}(\omega) = \sum_m \left[ -\frac{Y_{ia,m} X_{jb,m}^*}{\omega - \Omega_m + i\eta} + \frac{X_{ia,m}^* Y_{jb,m}}{\omega + \Omega_m - i\eta} \right], \quad \mathbf{i} L_{ia,jb}^{IV}(\omega) = \sum_m \left[ -\frac{Y_{ia,m} Y_{jb,m}^*}{\omega - \Omega_m + i\eta} + \frac{X_{ia,m}^* X_{jb,m}}{\omega + \Omega_m - i\eta} \right]. \quad (56)$$

It is straightforward to show that these blocks may be obtained if we define the operator  $L(\mathbf{x}_1 \mathbf{x}_2; \mathbf{x}_1' \mathbf{x}_2'; \omega)$  as

$$\mathbf{i} L(\mathbf{x}_1 \mathbf{x}_2; \mathbf{x}_1' \mathbf{x}_2'; \omega) = \sum_m \left[ -\frac{\rho_m(\mathbf{x}_1' \mathbf{x}_1) \rho_m^*(\mathbf{x}_2' \mathbf{x}_2)}{\omega - \Omega_m + i\eta} + \frac{\rho_m(\mathbf{x}_2' \mathbf{x}_2) \rho_m^*(\mathbf{x}_1' \mathbf{x}_1)}{\omega + \Omega_m - i\eta} \right], \quad (57)$$

where

$$\rho_m(\mathbf{x}_1' \mathbf{x}_1) = \sum_{ia} [X_{ia,m} \varphi_i^*(\mathbf{x}_1') \varphi_a(\mathbf{x}_1) + Y_{ia,m} \varphi_a^*(\mathbf{x}_1') \varphi_i(\mathbf{x}_1)]. \quad (58)$$

Before concluding this section, we emphasize the possibility of bypassing the diagonalization of the non-Hermitian matrix  $\mathcal{H}$  and instead determine  $X$  and  $Y$  via a Hermitian eigenproblem of half its original dimension, especially in the case of real-valued spin-orbitals. In fact, we have

$$\begin{aligned} \begin{pmatrix} A & B \\ -B & -A \end{pmatrix} \cdot \begin{pmatrix} X & Y \\ Y & X \end{pmatrix} &= \begin{pmatrix} X & Y \\ Y & X \end{pmatrix} \cdot \begin{pmatrix} \Omega & \mathbf{0} \\ \mathbf{0} & -\Omega \end{pmatrix} \Leftrightarrow \begin{cases} (A + B) \cdot (X + Y) = (X - Y) \cdot \Omega, \\ (A - B) \cdot (X - Y) = (X + Y) \cdot \Omega, \end{cases} \\ &\Leftrightarrow \begin{cases} (A + B) \cdot (A - B) \cdot (X - Y) = (X - Y) \cdot \Omega^2, \\ X + Y = (A - B) \cdot (X - Y) \cdot \Omega^{-1}. \end{cases} \end{aligned} \quad (59)$$

Supposing  $A - B$  positive definite, we can then insert  $(A - B)^{-1/2} \cdot (A - B)^{+1/2} = \mathbf{1}$  into the eigenproblem of  $X - Y$  and then multiply it on the left by  $(A - B)^{+1/2}$  to obtain the Hermitian eigenproblem

$$(A - B)^{1/2} \cdot (A + B) \cdot (A - B)^{1/2} \cdot \tilde{Z} = \tilde{Z} \cdot \Omega^2, \quad (60)$$

where  $\tilde{Z} = (A - B)^{+1/2} \cdot (X - Y)$ . To account for the normalization condition, we introduce the eigenvectors  $Z = \tilde{Z} \cdot \Omega^{-1/2}$ , which satisfy the same eigenproblem:

$$(A - B)^{1/2} \cdot (A + B) \cdot (A - B)^{1/2} \cdot Z = Z \cdot \Omega^2. \quad (61)$$

Hence, the matrices  $X$  and  $Y$  with the appropriate normalization are completely determined by these eigenvectors

$$\begin{cases} X - Y &= (A - B)^{-1/2} \cdot Z \cdot \Omega^{+1/2}, \\ X + Y &= (A - B)^{+1/2} \cdot Z \cdot \Omega^{-1/2}, \end{cases} \Leftrightarrow \begin{cases} X &= \frac{1}{2} \left[ (A - B)^{+1/2} \cdot Z \cdot \Omega^{-1/2} + (A - B)^{-1/2} \cdot Z \cdot \Omega^{+1/2} \right], \\ Y &= \frac{1}{2} \left[ (A - B)^{+1/2} \cdot Z \cdot \Omega^{-1/2} - (A - B)^{-1/2} \cdot Z \cdot \Omega^{+1/2} \right]. \end{cases} \quad (62)$$

## B. Screened interaction

Before computing the matrix elements of the various terms of the  $GW$  self-energy, we derive the matrix elements of the screened Coulomb interaction  $W$ . The expression of  $W(12; 1'2')$  is given by Eq. (30) and it can be written in terms of  $\tau = t_1 - t_2$  as

$$\begin{aligned} W(\mathbf{x}_1 \mathbf{x}_2; \mathbf{x}_1' \mathbf{x}_2'; \tau) &= v(\mathbf{x}_1 \mathbf{x}_2; \mathbf{x}_1' \mathbf{x}_2'; \tau) - i \int d(343'4') v(13; 1'3') L(4'3'; 4^+3^+) v(24; 2'4') \\ &= v(\mathbf{x}_1 \mathbf{x}_2; \mathbf{x}_1' \mathbf{x}_2'; \tau) - i \int d(\mathbf{x}_3 \mathbf{x}_4 \mathbf{x}_3' \mathbf{x}_4') v(\mathbf{x}_1 \mathbf{x}_3; \mathbf{x}_1' \mathbf{x}_3') v(\mathbf{x}_2 \mathbf{x}_4; \mathbf{x}_2' \mathbf{x}_4') L(\mathbf{x}_4' \mathbf{x}_3'; \mathbf{x}_4 \mathbf{x}_3; -\tau). \end{aligned} \quad (63)$$

Its Fourier transform is easy to compute and one gets

$$\begin{aligned} W(\mathbf{x}_1 \mathbf{x}_2; \mathbf{x}_1' \mathbf{x}_2'; \omega) &= \int d\tau e^{i\omega\tau} W(\mathbf{x}_1 \mathbf{x}_2; \mathbf{x}_1' \mathbf{x}_2'; \tau) \\ &= v(\mathbf{x}_1 \mathbf{x}_2; \mathbf{x}_1' \mathbf{x}_2') - i \int d(\mathbf{x}_3 \mathbf{x}_4 \mathbf{x}_3' \mathbf{x}_4') v(\mathbf{x}_1 \mathbf{x}_3; \mathbf{x}_1' \mathbf{x}_3') v(\mathbf{x}_2 \mathbf{x}_4; \mathbf{x}_2' \mathbf{x}_4') L(\mathbf{x}_4' \mathbf{x}_3'; \mathbf{x}_4 \mathbf{x}_3; -\omega) \\ &= v(\mathbf{x}_1 \mathbf{x}_2; \mathbf{x}_1' \mathbf{x}_2') + \sum_m \left[ \frac{M_m(\mathbf{x}_1 \mathbf{x}_1') M_m^*(\mathbf{x}_2 \mathbf{x}_2')}{\omega - \Omega_m + i\eta} - \frac{M_m^*(\mathbf{x}_1 \mathbf{x}_1') M_m(\mathbf{x}_2 \mathbf{x}_2')}{\omega + \Omega_m - i\eta} \right], \end{aligned} \quad (64)$$

where we have introduced the transition densities

$$\begin{aligned} M_m(\mathbf{x}_1 \mathbf{x}_1') &= \int d\mathbf{x}_2 d\mathbf{x}_2' v(\mathbf{x}_1 \mathbf{x}_2; \mathbf{x}_1' \mathbf{x}_2') \rho_m(\mathbf{x}_2 \mathbf{x}_2') \\ &= \int d\mathbf{x}_2 d\mathbf{x}_2' v(\mathbf{x}_1 \mathbf{x}_2; \mathbf{x}_1' \mathbf{x}_2') \rho_m(\mathbf{x}_2 \mathbf{x}_2) \\ &= M_m(\mathbf{x}_1 \mathbf{x}_1'). \end{aligned} \quad (65)$$

After projection in the spin-orbital basis, the matrix elements of  $W$  become

$$\begin{aligned} W_{rp,qs}(\omega) &= \int d\mathbf{x}_1 d\mathbf{x}_1' d\mathbf{x}_2 d\mathbf{x}_2' W(\mathbf{x}_1 \mathbf{x}_2; \mathbf{x}_1' \mathbf{x}_2'; \omega) \varphi_p^*(\mathbf{x}_1) \varphi_q^*(\mathbf{x}_2) \varphi_r(\mathbf{x}_1') \varphi_s(\mathbf{x}_2') \\ &= \langle pq|rs \rangle + \sum_m \left[ \frac{M_{pr,m} M_{sq,m}^*}{\omega - \Omega_m + i\eta} - \frac{M_{rp,m}^* M_{qs,m}}{\omega + \Omega_m - i\eta} \right], \end{aligned} \quad (66)$$

where we have introduced the elements of the transition densities

$$M_{pq,m} = \int d\mathbf{x}_1 d\mathbf{x}_1' M_m(\mathbf{x}_1 \mathbf{x}_1') \varphi_p^*(\mathbf{x}_1) \varphi_q(\mathbf{x}_1'). \quad (67)$$

Using the expression of  $\rho$  given in Eq. (58), the previous integral can be written as

$$M_{pq,m} = \sum_{ia} [X_{ia,m} \langle ap|i q \rangle + Y_{ia,m} \langle ip|a q \rangle]. \quad (68)$$

### C. GW self-energy

We now shift our focus to the calculation of the self-energy:

$$\Sigma_{xc}(11') = i \int d(22') G(22') W(12'; 21'), \quad (69)$$

where

$$W(12'; 21') = v(12'^-; 21') - i \int d(343'4') v(13; 23') L(4'3'; 4^+3^+) v(2'4; 1'4'). \quad (70)$$

By employing the expression for  $W$ , we can decompose this expression into separate exchange and correlation components, such that  $\Sigma_{xc}(11') = \Sigma_x(11') + \Sigma_c(11')$ , where the exchange part is

$$\begin{aligned} \Sigma_x(\mathbf{x}_1\mathbf{x}_{1'}; \tau_{11'} = t_1 - t_1') &= i \int d(22') G(22') v(12'^-; 21') \\ &= i \delta(\tau_{11'}) \int d(\mathbf{x}_2\mathbf{x}_{2'}) v(\mathbf{x}_1\mathbf{x}_{2'}; \mathbf{x}_2\mathbf{x}_{1'}) \int d(t_2t_{2'}) \delta(t_{2'} - \eta - t_{1'}) \delta(t_1 - t_2) G(\mathbf{x}_2\mathbf{x}_{2'}; t_2 - t_{2'}) \\ &= i \delta(\tau_{11'}) \int d(\mathbf{x}_2\mathbf{x}_{2'}) v(\mathbf{x}_1\mathbf{x}_{2'}; \mathbf{x}_2\mathbf{x}_{1'}) G(\mathbf{x}_2\mathbf{x}_{2'}; \tau_{11'} - \eta), \end{aligned} \quad (71)$$

and the correlation part is

$$\begin{aligned} \Sigma_c(\mathbf{x}_1\mathbf{x}_{1'}; \tau_{11'}) &= \int d(2342'3'4') G(22') v(13; 23') L(4'3'; 4^+3^+) v(2'4; 1'4') \\ &= \int d(\mathbf{x}_2\mathbf{x}_3\mathbf{x}_4\mathbf{x}_{2'}\mathbf{x}_{3'}\mathbf{x}_{4'}) v(\mathbf{x}_1\mathbf{x}_3; \mathbf{x}_2\mathbf{x}_{3'}) v(\mathbf{x}_{2'}\mathbf{x}_4; \mathbf{x}_{1'}\mathbf{x}_{4'}) \\ &\quad \times \int d(t_2t_3t_4t_{2'}t_{3'}t_{4'}) \delta(t_1 - t_2) \delta(t_1 - t_{3'}) \delta(t_3 - t_{3'}) \delta(t_{2'} - t_{1'}) \delta(t_4 - t_{4'}) \delta(t_{2'} - t_{4'}) \\ &\quad \times G(\mathbf{x}_2\mathbf{x}_{2'}; t_2 - t_{2'}) L(4'3'; 4^+3^+) \\ &= \int d(\mathbf{x}_2\mathbf{x}_3\mathbf{x}_4\mathbf{x}_{2'}\mathbf{x}_{3'}\mathbf{x}_{4'}) v(\mathbf{x}_1\mathbf{x}_3; \mathbf{x}_2\mathbf{x}_{3'}) v(\mathbf{x}_{2'}\mathbf{x}_4; \mathbf{x}_{1'}\mathbf{x}_{4'}) G(\mathbf{x}_2\mathbf{x}_{2'}; \tau_{11'}) L(\mathbf{x}_4\mathbf{x}_{3'}; \mathbf{x}_4\mathbf{x}_3; -\tau_{11'}). \end{aligned} \quad (72)$$

The exchange self-energy does not depend on  $\tau$ . Hence, its Fourier transform is trivial and one gets

$$\begin{aligned} \Sigma_x(\mathbf{x}_1\mathbf{x}_{1'}; \omega) &= \int d\tau_{11'} e^{i\omega\tau_{11'}} \Sigma_x(\mathbf{x}_1\mathbf{x}_{1'}; \tau_{11'}) \\ &= i \int d(\mathbf{x}_2\mathbf{x}_{2'}) v(\mathbf{x}_1\mathbf{x}_{2'}; \mathbf{x}_2\mathbf{x}_{1'}) \int d\tau_{11'} e^{i\omega\tau_{11'}} \delta(\tau_{11'}) G(\mathbf{x}_2\mathbf{x}_{2'}; \tau_{11'} - \eta) \\ &= i \int d(\mathbf{x}_2\mathbf{x}_{2'}) v(\mathbf{x}_1\mathbf{x}_{2'}; \mathbf{x}_2\mathbf{x}_{1'}) \int d\tau_{11'} e^{i\omega\tau_{11'}} \delta(\tau_{11'}) \frac{1}{2\pi} \int d\omega' e^{-i\omega'(\tau_{11'} - \eta)} G(\mathbf{x}_2\mathbf{x}_{2'}; \omega') \\ &= i \int d(\mathbf{x}_2\mathbf{x}_{2'}) v(\mathbf{x}_1\mathbf{x}_{2'}; \mathbf{x}_2\mathbf{x}_{1'}) \frac{1}{2\pi} \int d\omega' e^{i\omega'\eta} G(\mathbf{x}_2\mathbf{x}_{2'}; \omega') \\ &= i \int d(\mathbf{x}_2\mathbf{x}_{2'}) v(\mathbf{x}_1\mathbf{x}_{2'}; \mathbf{x}_2\mathbf{x}_{1'}) \frac{1}{2\pi} \int d\omega' e^{i\omega'\eta} \left[ \sum_i \frac{\varphi_i(\mathbf{x}_2) \varphi_i^*(\mathbf{x}_{2'})}{\omega' - (\epsilon_i + i\eta)} + \sum_a \frac{\varphi_a(\mathbf{x}_2) \varphi_a^*(\mathbf{x}_{2'})}{\omega' - (\epsilon_a - i\eta)} \right] \\ &= - \int d(\mathbf{x}_2\mathbf{x}_{2'}) v(\mathbf{x}_1\mathbf{x}_{2'}; \mathbf{x}_2\mathbf{x}_{1'}) \varphi_i(\mathbf{x}_2) \varphi_i^*(\mathbf{x}_{2'}). \end{aligned} \quad (73)$$

The Fourier transform of the correlation self-energy reads

$$\begin{aligned} \Sigma_c(\mathbf{x}_1\mathbf{x}_{1'}; \omega) &= \int d\tau_{11'} e^{i\omega\tau_{11'}} \Sigma_c(\mathbf{x}_1\mathbf{x}_{1'}; \tau_{11'}) \\ &= \int d\tau_{11'} e^{i\omega\tau_{11'}} \int d(\mathbf{x}_2\mathbf{x}_3\mathbf{x}_4\mathbf{x}_{2'}\mathbf{x}_{3'}\mathbf{x}_{4'}) v(\mathbf{x}_1\mathbf{x}_3; \mathbf{x}_2\mathbf{x}_{3'}) v(\mathbf{x}_{2'}\mathbf{x}_4; \mathbf{x}_{1'}\mathbf{x}_{4'}) G(\mathbf{x}_2\mathbf{x}_{2'}; \tau_{11'}) L(\mathbf{x}_4\mathbf{x}_{3'}; \mathbf{x}_4\mathbf{x}_3; -\tau_{11'}) \\ &= \int d(\mathbf{x}_2\mathbf{x}_3\mathbf{x}_4\mathbf{x}_{2'}\mathbf{x}_{3'}\mathbf{x}_{4'}) v(\mathbf{x}_1\mathbf{x}_3; \mathbf{x}_2\mathbf{x}_{3'}) v(\mathbf{x}_{2'}\mathbf{x}_4; \mathbf{x}_{1'}\mathbf{x}_{4'}) \int \frac{d\omega''}{2\pi} G(\mathbf{x}_2\mathbf{x}_{2'}; \omega'') \int \frac{d\omega'}{2\pi} L(\mathbf{x}_4\mathbf{x}_{3'}; \mathbf{x}_4\mathbf{x}_3; \omega') \underbrace{\int d\tau_{11'} e^{i(\omega - \omega'' + \omega')\tau_{11'}}}_{2\pi\delta(\omega - \omega'' + \omega')} \\ &= \int d(\mathbf{x}_2\mathbf{x}_3\mathbf{x}_4\mathbf{x}_{2'}\mathbf{x}_{3'}\mathbf{x}_{4'}) v(\mathbf{x}_1\mathbf{x}_3; \mathbf{x}_2\mathbf{x}_{3'}) v(\mathbf{x}_{2'}\mathbf{x}_4; \mathbf{x}_{1'}\mathbf{x}_{4'}) \int \frac{d\omega'}{2\pi} L(\mathbf{x}_4\mathbf{x}_{3'}; \mathbf{x}_4\mathbf{x}_3; \omega') G(\mathbf{x}_2\mathbf{x}_{2'}; \omega + \omega'). \end{aligned} \quad (74)$$

The integral over  $\omega'$  gives

$$\begin{aligned}
& \int \frac{d\omega'}{2\pi} L(\mathbf{x}_4' \mathbf{x}_3'; \mathbf{x}_4 \mathbf{x}_3; \omega') G(\mathbf{x}_2 \mathbf{x}_2'; \omega + \omega') \\
&= (-i) \int \frac{d\omega'}{2\pi} \sum_m \left[ -\frac{\rho_m(\mathbf{x}_4 \mathbf{x}_4') \rho_m^*(\mathbf{x}_3' \mathbf{x}_3)}{\omega' - \Omega_m + i\eta} + \frac{\rho_m(\mathbf{x}_3 \mathbf{x}_3') \rho_m^*(\mathbf{x}_4' \mathbf{x}_4)}{\omega' + \Omega_m - i\eta} \right] \left[ \sum_i \frac{\varphi_i(\mathbf{x}_2) \varphi_i^*(\mathbf{x}_2')}{\omega + \omega' - \epsilon_i - i\eta} + \sum_a \frac{\varphi_a(\mathbf{x}_2) \varphi_a^*(\mathbf{x}_2')}{\omega + \omega' - \epsilon_a + i\eta} \right] \\
&= \sum_{m,i} \frac{\rho_m(\mathbf{x}_4 \mathbf{x}_4') \rho_m^*(\mathbf{x}_3' \mathbf{x}_3) \varphi_i(\mathbf{x}_2) \varphi_i^*(\mathbf{x}_2')}{\omega + \Omega_m - \epsilon_i - 2i\eta} + \sum_{m,a} \frac{\rho_m(\mathbf{x}_3 \mathbf{x}_3') \rho_m^*(\mathbf{x}_4' \mathbf{x}_4) \varphi_a(\mathbf{x}_2) \varphi_a^*(\mathbf{x}_2')}{\omega - \Omega_m - \epsilon_a + 2i\eta}.
\end{aligned} \tag{75}$$

Hence, the correlation part of the self-energy becomes

$$\Sigma_c(\mathbf{x}_1 \mathbf{x}_1'; \omega) = \int d\mathbf{x}_2 d\mathbf{x}_2' \left[ \sum_{m,i} \frac{M_m^*(\mathbf{x}_1 \mathbf{x}_2) M_m(\mathbf{x}_2' \mathbf{x}_1') \varphi_i(\mathbf{x}_2) \varphi_i^*(\mathbf{x}_2')}{\omega + \Omega_m - \epsilon_i - 2i\eta} + \sum_{m,a} \frac{M_m(\mathbf{x}_1 \mathbf{x}_2) M_m^*(\mathbf{x}_2' \mathbf{x}_1') \varphi_a(\mathbf{x}_2) \varphi_a^*(\mathbf{x}_2')}{\omega - \Omega_m - \epsilon_a + 2i\eta} \right]. \tag{76}$$

The matrix elements of the self-energy are obtained as

$$[\Sigma_x(\omega)]_{pq} = \int d\mathbf{x}_1 d\mathbf{x}_1' \Sigma_x(\mathbf{x}_1 \mathbf{x}_1'; \omega) \varphi_p^*(\mathbf{x}_1) \varphi_q(\mathbf{x}_1') = - \sum_i \langle p | i | q \rangle, \tag{77}$$

and

$$[\Sigma_c(\omega)]_{pq} = \int d\mathbf{x}_1 d\mathbf{x}_1' \Sigma_c(\mathbf{x}_1 \mathbf{x}_1'; \omega) \varphi_p^*(\mathbf{x}_1) \varphi_q(\mathbf{x}_1') = \sum_{m,i} \frac{M_{pi,m}^* M_{qi,m}}{\omega + \Omega_m - \epsilon_i - i\eta} + \sum_{m,a} \frac{M_{pa,m} M_{qa,m}^*}{\omega - \Omega_m - \epsilon_a + i\eta}. \tag{78}$$

#### D. GW correlation energies

Let us first recall the equation of motion

$$i \frac{\partial}{\partial t_1} G(11') - h(\mathbf{x}_1) G(11') - \int d3 \Sigma(13) G(31') = \delta(11'). \tag{79}$$

where a local one-body potential  $h$  is considered here because the kinetic and nuclear repulsion potentials are both local. As derived in Fetter's and Walecka's book,<sup>5</sup> the Galitskii-Migdal (GM) functional is

$$\begin{aligned}
E^{\text{GM}} &= -\frac{i}{2} \int d\mathbf{x}_1 \lim_{2 \rightarrow 1^+} \left[ i \frac{\partial}{\partial t_1} + h(\mathbf{x}_1) \right] G(12) \\
&= -\frac{i}{2} \int d\mathbf{x}_1 \lim_{2 \rightarrow 1^+} i \frac{\partial G(12)}{\partial t_1} - \frac{i}{2} \int d\mathbf{x}_1 \lim_{2 \rightarrow 1^+} h(\mathbf{x}_1) G(12) \\
&= -\frac{i}{2} \int d\mathbf{x}_1 \lim_{2 \rightarrow 1^+} \left[ \delta(12) + h(\mathbf{x}_1) G(12) + \int d3 \Sigma(13) G(32) \right] - \frac{i}{2} \int d\mathbf{x}_1 \lim_{2 \rightarrow 1^+} h(\mathbf{x}_1) G(12) \\
&= -\frac{i}{2} \int d\mathbf{x}_1 \lim_{2 \rightarrow 1^+} \underbrace{\delta(12)}_{=0} - i \int d\mathbf{x}_1 \lim_{2 \rightarrow 1^+} \left[ h(\mathbf{x}_1) G(12) + \frac{1}{2} \int d3 \Sigma(13) G(32) \right] \\
&= -i \int d\mathbf{x}_1 \lim_{2 \rightarrow 1^+} \left[ h(\mathbf{x}_1) G(12) + \frac{1}{2} \int d3 \Sigma(13) G(32) \right]
\end{aligned}$$

which can be further separated as

$$\begin{aligned}
E^{\text{GM}} &= -i \int d\mathbf{x}_1 \lim_{2 \rightarrow 1^+} \left[ h(\mathbf{x}_1) G(12) + \frac{1}{2} \int d3 \Sigma_{\text{Hx}}(13) G(32) \right] - \frac{i}{2} \int d\mathbf{x}_1 \lim_{2 \rightarrow 1^+} \int d3 \Sigma_c(13) G(32) \\
&= E_{\text{Hx}}^{\text{GM}} + E_c^{\text{GM}}
\end{aligned}$$

The first term is equal to the HF energy, i.e.  $E_{\text{Hx}}^{\text{GM}} = E_{\text{HF}}$ , if evaluated with the HF Green's function. Let us now focus on the correlation energy which reads

$$\begin{aligned}
E_c^{\text{GM}} &= -\frac{i}{2} \int d\mathbf{x}_1 \lim_{2 \rightarrow 1^+} \int d3 \Sigma_c(13) G(32) \\
&= -\frac{i}{2} \int d\mathbf{x}_1 \lim_{2 \rightarrow 1^+} \int d3 \Sigma_c(13) \int \frac{d\omega}{2\pi} e^{-i\omega(t_3-t_2)} G(\mathbf{x}_3 \mathbf{x}_2; \omega) \\
&= -\frac{i}{2} \int d\mathbf{x}_1 \lim_{2 \rightarrow 1^+} \int \frac{d\omega}{2\pi} e^{i\omega(t_2-t_1)} \int d3 e^{i\omega(t_1-t_3)} \Sigma_c(13) G(\mathbf{x}_3 \mathbf{x}_2; \omega) \\
&= -\frac{i}{2} \int d\mathbf{x}_1 \int \frac{d\omega}{2\pi} \lim_{2 \rightarrow 1^+} e^{i\omega(t_2-t_1)} \int d\mathbf{x}_3 \Sigma_c(\mathbf{x}_1 \mathbf{x}_3; \omega) G(\mathbf{x}_3 \mathbf{x}_2; \omega) \\
&= -\frac{i}{2} \int d\mathbf{x}_1 \int \frac{d\omega}{2\pi} e^{i\omega\eta} \int d\mathbf{x}_3 \Sigma_c(\mathbf{x}_1 \mathbf{x}_3; \omega) G(\mathbf{x}_3 \mathbf{x}_1; \omega)
\end{aligned}$$

The last step consists of transforming the previous equation into an implementable version involving matrix elements. This yields

$$\begin{aligned}
E_c^{\text{GM}} &= -\frac{i}{2} \int \frac{d\omega}{2\pi} e^{i\omega\eta} \int d\mathbf{x}_1 \int d\mathbf{x}_3 \left( \sum_{pq} \varphi_p^*(\mathbf{x}_1) \varphi_q(\mathbf{x}_3) [\Sigma_c(\omega)]_{pq} \right) \left( \sum_{rs} \varphi_r^*(\mathbf{x}_3) \varphi_s(\mathbf{x}_1) G_{rs}(\omega) \right) \\
&= -\frac{i}{2} \int \frac{d\omega}{2\pi} e^{i\omega\eta} \sum_{pq} [\Sigma_c(\omega)]_{pq} G_{qp}(\omega) \\
&= -\frac{i}{2} \int \frac{d\omega}{2\pi} e^{i\omega\eta} \sum_{pq} \left( \sum_{mi} \frac{M_{pi,m}^* M_{qi,m}}{\omega - (\epsilon_i - \Omega_m + i\eta)} + \sum_{ma} \frac{M_{pa,m} M_{qa,m}^*}{\omega - (\epsilon_a + \Omega_m - i\eta)} \right) \left( \sum_j \frac{\delta_{pqj}}{\omega - (\epsilon_j + i\eta)} + \sum_b \frac{\delta_{pqb}}{\omega - (\epsilon_b - i\eta)} \right) \\
&= \frac{1}{2} \sum_{pq} \left( \sum_{mib} \frac{M_{pi,m}^* M_{qi,m} \delta_{pqb}}{(\epsilon_i - \Omega_m + i\eta) - (\epsilon_b - i\eta)} + \sum_{maj} \frac{M_{pa,m} M_{qa,m}^* \delta_{pqj}}{(\epsilon_j + i\eta) - (\epsilon_a + \Omega_m - i\eta)} \right) \\
&= -\frac{1}{2} \sum_{mia} \frac{M_{ai,m}^* M_{ai,m}}{\epsilon_a - \epsilon_i + \Omega_m - 2i\eta} - \frac{1}{2} \sum_{mai} \frac{M_{ia,m} M_{ia,m}^*}{\epsilon_a - \epsilon_i + \Omega_m + 2i\eta}
\end{aligned}$$

## Acknowledgments

This project has received financial support from the European Research Council (ERC) under the European Union's Horizon 2020 research and innovation programme (Grant agreement No. 863481) for funding. Additionally, it was supported by the European Centre of Excellence in Exascale Computing (TREX), and has received funding from the European Union's Horizon 2020 — Research and Innovation program — under grant agreement no. 952165.

## References

- <sup>1</sup>L. Kadanoff and G. Baym, *Quantum Statistical Mechanics: Green's Function Methods in Equilibrium and Nonequilibrium Problems*, Frontiers in Physics. A Lecture Note and Reprint Series (W.A. Benjamin, 1962).
- <sup>2</sup>R. M. Martin, L. Reining, and D. M. Ceperley, *Interacting Electrons: Theory and Computational Approaches* (Cambridge University Press, 2016).
- <sup>3</sup>J. Schirmer, *Many-Body Methods for Atoms, Molecules and Clusters* (Springer Cham, 2018).
- <sup>4</sup>A. Szabo and N. S. Ostlund, *Modern quantum chemistry* (McGraw-Hill, New York, 1989).
- <sup>5</sup>A. L. Fetter and J. D. Walecka, *Quantum Theory of Many Particle Systems* (McGraw Hill, San Francisco, 1971).
